# Supplementary material for: VALL-E R: Robust and Efficient Zero-Shot Text-to-Speech Synthesis via Monotonic Alignment
Source: arXiv:2406.07855 source file (2024-06-12)
Supplement: Supplementary file 1 [file appendix.tex]

\appendix

\section{Some Examples of Training Data}
\subsection{SQA Task}\label{App_A_1}
\par
\begin{tabular}
{p{6cm}|p{4cm}|p{3cm}|p{1.5cm}}
\hline\hline
speech transcript                                                & instructions                                                                                               & targets                                                                              & source       \\ 
\hline
the nautilus would still have nothing to fear from their attacks & What animal would still have nothing to fear from attacks? & The nautilus. & LibriSpeech \\
\hline
as gelatinous or glutinous matters impress the sense of touch i have spoken both of sound and of voice i mean to say that the sound was one of distinct of even wonderfully thrillingly distinct & What is the gender of the speaker? And what is the speaker talking about? & The speaker is female. And she is talking about sound and voice being distinct. & LibriSpeech \\
\hline
A: so how do you feel about it; B: uh i don't see any problem with with random- testing for random drugs; A: yeah i myself almost um am in favor of it uh; A: i work at Honeywell and i went through a a pretty i don't know i went through a standard drug testing thing before i was brought on; B: um-hum & What is the second speaker's opinion on random drug testing? & The second speaker doesn't see any problem with random drug testing. & Switchboard \\
\hline\hline
\end{tabular}

\subsection{Multi-task Instruction Datasets}\label{App_A_2}
\par
\begin{tabular}{p{4cm}|p{4cm}|p{5cm}|p{1.5cm}}
\hline\hline
speech transcript                                                & instructions                                                                                               & targets                                                                              & source       \\ 
\hline
the nautilus would still have nothing to fear from their attacks & Initially, Analyze the speech in the given audio clip and provide a complete textual transcription; Then, answer the question: What animal would still have nothing to fear from attacks?; Thirdly, ignore the audio clip, Come up with 5 activities for a birthday party for a 5-year-old. & The audio transcription is: the nautilus would still have nothing to fear from their attacks \textbackslash{}n For the question ``{}What animal would still have nothing to fear from attacks?'', the response is: The nautilus. \textbackslash{}n The response to ``{}Come up with 5 activities for a birthday party for a 5-year-old. '' is: 1. Play a game of freeze dance \textbackslash{}n 2. Make balloon animals \textbackslash{}n 3. Have a color scavenger hunt \textbackslash{}n 4. Bake cupcakes  \textbackslash{}n 5. Make a craft project together & LibriSpeech, Alpaca \\
\hline\hline
\end{tabular}

\subsection{The Prompts for Generating SQA Data by GPT-4}\label{App_A_3}

\begin{tabular}{p{16cm}}
\hline\hline
You are asked to generate **only one** questions, and their corresponding answers, according to some conversational sentences given below. These sentences have been transcribed from conversational speech data with one or multiple speakers who are taking to each other. ``Speaker A'' and ``Speaker B'' in the senteces are labeled by human and your response must not contain human-marked information, namely ``Speaker A'' and ``Speaker B''. Here are the requirements: 1. Your response should strictly follow the format below: {``Question'': ``xxx'', ``Answer'': ``xxx''}; 2. Please ignore ``Speaker A'' and ``Speaker B'' in the given sentences. Your response should strictly not include the phrase ``Speaker A'' and ``Speaker B''; 3. Your question should be highly related to the conversation, and your answer must be **correct**, and should be simple and clear. Besides, you question should be designed as your answer has to be reasoned from the conversation; 4. For example, a sentence ``Speaker A: It is a good day; Speaker B: Yes, but I have to go to hospital'' means that speaker A first say it is a good day and speaker B then say that Yes, but I have to go to hospital. 5. **Very Importance**: Your questions and answers **can not** contain the word ``Speaker A'' and ``Speaker B'', because ``Speaker A'' and ``Speaker B'' in the sentences are additional labels for transcripts, and they are different people. For example, the question ``What is Speaker B's opinion?'' **does not** meet the requirements because it contains word ``Speaker B''. Namely, you can not use ``Speaker A'' and ``Speaker B'' to represent they in questions and answers, maybe you can use the first or second speaker to denote ``Speaker A'' or ``Speaker B''; 6. The type of response should be diverse. The respone **must contain** double quotation marks for each part. Here are the sentences: {transcript}
\\
\hline\hline
\end{tabular}

\section{Some Examples of Evaluation Data}\label{App_B}

\subsection{Examples of II-task Instruction}\label{App_B_1}
\par
\begin{tabular}{p{4cm}|p{8cm}|p{1cm}|p{1.5cm}}
\hline\hline
speech transcript                                                & instructions                                                                                               & targets                                                                              & source       \\ 
\hline
Women: ``How much time do you usually spend exercising daily?'' 
Man: ``Frankly speaking, I'm an awfully lazy man. I know it's time to change.'' & To begin, What will the man do next? A. Start to take exercise; B. Do as he always does; C. Change his working time.; Next, Create a French transcript for this English audio clip; Furthermore, Recognize the speech and give me the transcription; Last step, setting aside the audio, Who wrote ``The Adventures of Sherlock Holmes''? & - & MuTual  \\
\hline\hline
\end{tabular}

\subsection{Examples of CoT-task and Non-CoT-task Instruction}\label{App_B_2}
\par
\begin{tabular}{p{5.5cm}|p{6cm}|p{2cm}|p{1cm}}
\hline\hline
speech transcript                                                & instructions                                                                                               & targets                                                                              & source       \\ 
\hline
three films from Asia-Pacific are in the running for the coveted golden palms at this year\'s Cannes film festival, competing in a field dominated by European productions, organizers announced Monday.   &  First of all, transcribe the audio recording into text, capturing every spoken word; Additionally given this audio clip and text, can you condense it into a clear, concise summary, no more than 20 words?; Lastly disregarding the sound, translate this English summary into German. & Drei Filme aus dem asiatisch-pazifischen Raum im Rennen in Cannes & gigaword \\
\hline
three films from Asia-Pacific are in the running for the coveted golden palms at this year\'s Cannes film festival, competing in a field dominated by European productions, organizers announced Monday.   &  Please summarize the content of the audio clip in German, no more than 20 words. & Drei Filme aus dem asiatisch-pazifischen Raum im Rennen in Cannes & gigaword \\
\hline\hline
\\
\end{tabular}

\section{The Prompt for Scoring using GPT-4}
\subsection{SQA Scoring}\label{App_C_1}
\begin{tabular}{p{16cm}}
\hline\hline
Next, I will give you a multiple-choice question along with its correct answer, as well as a generated answer that needs to be evaluated for correctness. You will need to determine whether the given answer is correct based on the question and the correct answer, and give a simple reason. The answer must explicitly give the correct option to be considered correct and not by implication or indirect response. Your response should strictly follow the format:\{"result": "xx", "reason": "xx"\}, if the given answer is correct, then your response should be \{"result": "True", "reason": "xx"\}, otherwise your response should be \{"result": "False", "reason": "xx"\}.Here is the question: \{"What will the man do next? A. Start to take exercise; B. Do as he always does; C. Change his working time."\},and the correct answer is \{"A"\},the answer that needs to be judged is \{"B. Do as he always does"\}.
\\
\hline\hline
\end{tabular}

\subsection{II-task Scoring}\label{App_C_2}
\begin{tabular}{p{16cm}}
\hline\hline
Next i will give you an audio transcription, instructions related or unrelated to the audio, and the corresponding responses. You need to use the given information to figure out how many instructions were completed correctly in the given responses and how many were left unanswered or answered incorrectly, then give the simple and clear reason why each question was completed or not, Finally, you need to do the self-examination to ensure responses you give must be correct and without inconsistencies.\\You must adhere to the following \textbf{rules}: 1. instructions are only answered sequentially, and one answer must only correspond to one instruction; 2. For choice questions, the answer must be in **English** and only **one** of the three options, multiple options or none of the options are considered incomplete, e.g. the answer is ``A. xx; B. xx; C. xx.'' (note that options may appear across sentences or lines); 3. All instructions must be completed in **English**, except translation tasks; 4. The translation task is not a translation of instructions, but a translation of the content of the given audio speech 5. If the response is a repetition of the instruction, then it is considered not completed.\\Your response should strictly follow the format: \{``instructions completed'': ``xx'', ``instructions incompleted'': ``xx'', ``Reasons for each instructions'': [``instruction\_1: xx'', ``instruction\_2: xx'', ``instruction\_3: xx'', ``instruction\_4: xx'']\}.
\\
\hline
You need to refer to \textbf{this example}: the transcription of the audio: ``So James What are you going to do for your birthday? Well, I was hoping to have a party but most of my friends are busy so I have accepted my sisters offer to take me to a film. At least it is better than going out for a meal with my parents.''; the instructions are ``To begin, ignore the audio clip, Who is known for developing the theory of relativity?; Then, What will the man do on his birthday? A. Have a party; B. See a movie; C. Go out for a meal.; Moreover, Convert the spoken words in this audio file into a textual format; Last step, Translate this English speech into Japanese";\\and the respones are ``1. \begin{CJK*}{UTF8}{min}
エイトリングの理論を発展した人物は誰ですか？
\end{CJK*}; 2. What will the man do on his birthday? A. Have a party; B. See a movie; C. Go out for a meal.; 3. \begin{CJK*}{UTF8}{min}この音声>ファイルをテキスト形式に変換してください。\end{CJK*}; 4.  \begin{CJK*}{UTF8}{min}この英語のスピーチを日本語に翻訳してください。\end{CJK*}''.\\And your output should be \{``instructions completed'': ``0'', ``instructions incompleted'': ``4'', ``Reasons for each instructions'': [``instruction\_1: incompleted, the answer is the Japanese translation of the instruction. Q\&A task should be completed in English.'', ``instruction\_2: incompleted, the answer is the a repetition of the instruction. More than one options were given'', ``instruction\_3: incompleted, the answer is the Japanese translation of the instruction'', ``instruction\_4: incompleted, the answer is the Japanese translation of the instruction'']\}.\\Be sure to carefully follow the rules and refer to the examples for responses.\\
\hline
\textbf{Here is the transcription of the audio}: \{``I really want to go to the concert, but I haven't got a ticket yet leave it to me, I'll organize that we can go together really that's wonderful.''\},\\ \textbf{the instructions} are \{``To begin, disregarding the sound, How many elements are on the periodic table?; Then, Translate this English speech into Japanese; Additionally, How will the speaker get a ticket to the concert? A. The man will go to buy the ticket; B. The woman will get the ticket; C. The man will have someone buy the ticket.; Lastly, Transcribe the given audio clip into text''\},\\\textbf{the responses} is \{``Addressing the prompt 'How many elements are on the periodic table?', the answer is: There are currently 118 elements on the periodic table. From the audio, we have the following translations: \begin{CJK*}{UTF8}{min}コンサートに行きたいけど まだチケットがないの どうするんだ？\end{CJK*} For the question ``How will the speaker get a ticket to the concert? A. The man will go to buy the ticket; B. The woman will get the ticket; C. The man will have someone buy the ticket.'', the response is: B; The audio transcription is: i really want to go to the concert but i haven't got a ticket yet b  leave it to me i'll organize that we can go together r  really that's wonderful \}
\\
\hline\hline
\end{tabular}

\section{Prompt Template for WavLLM}\label{App_D}
The template of our WavLLM containing a speech audio clip, text instructions and targets are constructed as follows: \\
\\
\begin{tabular}{p{16cm}}
\hline
\textless bos\textgreater\lbrack INST\rbrack\textless\textless SYS\textgreater\textgreater\textbackslash n As a helpful language and speech assistant, you are able to understand the speech content provided by the user, and assist the user with a variety of tasks using natural language. \textbackslash n\textless\textless/SYS\textgreater\textgreater\textbackslash n\textbackslash n \textless SPEECH\textgreater `` speech '' \textless/SPEECH\textgreater``instruction'' \lbrack/INST\rbrack`` target ''\textless eos\textgreater \\
\hline
\end{tabular}
\\
\\
where ``speech'' will be replaced by the 4096-dim speech features extracted from speech encoders and modality adapters, while ``instruction'' and ``target'' are the specific task prompts and outputs. The input to the WavLLM is this template with the <eos> removed, while the target is this template without the <bos>. During training, only the ``target'' part is involved in the loss calculation.

\section{Example of Multi-round Dialog}\label{App_E}
\begin{figure}[H]
    \centering
    \includegraphics[width=12cm]{figure/case.pdf}
    \caption{An example of multi-round dialog based on Gaokao task}
    \label{fig:enter-label}
\end{figure}
